# Supplementary material for: An authenticated and secure accounting system for international emissions trading
Source: arXiv:2011.13954 source file (2020-11-27)
Supplement: Supplementary file 1 [file appendix.tex]

% !TEX root = main.tex

\section{Formalized protocols}

Here we provide a formal presentation of all the cryptographic protocols discussed in the main text. We first formalize the commitment scheme. An auditing protocol $\Pi_\audit$ that integrates the entire reporting and the verification process is then presented, assuming there exists a protocol that can generate a random list for verification. This random list generation protocol is also formalized as protocol $\Pi_\pick$. 

\subsection{Commitment}
A \emph{commitment scheme} can be represented by a tuple of two algorithms $(\stp,\comm)$ defined as follows:
\begin{itemize}
    \item $pp\leftarrow\stp(1^\kappa)$ takes a security parameter $\kappa$ and outputs public parameter $pp$ for commitment.
    \item $c\leftarrow\comm_{pp}(m,r)$ commits a message $m$ in the message space $\cal M$ with a random value $r$ from random value space $\cal R$. The message space $\cal M$ and random value space $\cal R$ are specified in $pp$.
\end{itemize}

\begin{define}
    $(\stp,\comm)$ is a secure additive commitment scheme if it satisfy the following properties.
    \begin{itemize}
        \item \textbf{(Unconditional hiding)}  For any $m_1,m_2\in {\cal M}$ and $r_1,r_2$ picked uniformly random from $\cal R$, $\comm_{pp}(m_1,r_1)$ and $\comm_{pp}(m_2,r_2)$ has the same probability distribution.
        \item \textbf{(Computational biding)} For any probabilistic polynomial time adversary $\cal A$, $$\Pr\left[\begin{array}{l}
            pp\leftarrow\stp(1^\kappa),(m_1,m_2,r_1,r_2)\leftarrow {\cal A}(pp):  \\
            (m_1\neq m_2\;\vee\;r_1\neq r_2)\;\wedge\;\comm_{pp}(m_1,r_1) = \comm_{pp}(m_2,r_2) 
        \end{array} \right]\le \epsilon(\kappa)$$
        where $\epsilon(\cdot)$ is a negligible function. 
        \item \textbf{(Additive)}  For any $m_1,m_2\in {\cal M}$ and $r_1,r_2\in {\cal R}$,  $\comm_{pp}(m_1,r_1) + \comm_{pp}(m_2,r_2)=\comm_{pp}(m_1+m_2,r_1+r_2)$.
        
    \end{itemize}
\end{define}

\paragraph{Construction}

The $\stp(1^\kappa)$ algorithm takes the security parameter $\kappa$ as input and outputs public parameter $pp$. $pp$ contains an elliptic curve group $\mathbb{G}$ with  security bits $\kappa$ and a starting point $G$, in which the ECDLP (Elliptic Curve Discrete Logarithm Problem) is hard to solve. The order of this group is a large prime integer $q$. The message space $\cal M$ and the random value space $\cal R$ are $\mathbb{Z}_q$. $pp$ also contains a point $H$ on the elliptic curve. 

The $\comm_{pp}(m,r)$ algorithm takes a message $m\in {\cal M}$ and a random value $r \in {\cal R}$ as input, and outputs $m\cdot G+r\cdot H$ as the committed message. The notations have been defined in section ``Constructing protocols''.

This construction is called the \emph{Pedersen commitment scheme} and has been proved a secure additive commitment scheme in~\cite{pedersen1991non}. 

\subsection{Auditing Protocol}

The auditing protocol $\Pi_\audit$ models our hiding and binding protocol and verifiable summation protocol together. $\Pi_{\audit}$ consists of an environment $E$ and a set $\cal P$ of the following participants: $n$ firms $\{F_i\}_{i=1}^n$, the country $C$ and the verifier $V$.

Before executing the protocol, the environment $E$ runs an algorithm $\mathsf{Env}(\kappa,k)$ which outputs public parameters for commitment $pp=\stp(1^\kappa)$, the real carbon emission data $m_i\in {\cal M}$ for each firm $F_i$ and an uniformly random subset $\cal V$ with $k$ firms. The environment stores these outputs locally.

\paragraph{Construction} 
This protocol is designed based on a secure additive commitment schemes. We also assume there is a broadcast channel shared by all the participants. Such a channel can prevent the adversary from sending different messages to different participants when broadcasting one message. The protocol is executed as the following steps. 

\begin{enumerate}
    \item The environment $E$ broadcasts $pp$ and forwards $m_i$ to firm $F_i$.
    \item The firm $F_i$ picks random $r_i$ from $\cal R$ and computes $c_i=\comm_{pp}(m_i,r_i)$. It broadcasts $c_i$ and forwards $m_i,r_i$ to the country $C$. 
    \item The country $C$ examines whether $c_i=\comm_{pp}(m_i,r_i)$ for all the $i\in[n]$.
    \item The country broadcasts $m=\sum_i m_i$ and $r=\sum_i r_i$. 
    \item The environment $E$ broadcasts $\cal V$. For each picked firm $F_i\in {\cal V}$, the environment $E$ forwards $m_i$ to the verifier and the firm $F_i$ forwards $r_i$ to the verifier. 
    \item For each picked firm $F_i$, the verifier $V$ examines $c_i=\comm_{pp}(m_i,r_i)$. 
    \item The verifier $V$ examines whether $\sum_i c_i=\comm_{pp}(m,r)$.  
\end{enumerate}

During the execution of the protocol, whenever the examination fails, the protocol execution fails. 

In this construction, the random firm list is generated at the beginning and kept invisible from all the participants until step 5. It is equivalent to generate such a random list after step 4. We model picking the random list as an environment setup process for convenience in the subsequent analysis.

\paragraph{Adversary model} In this protocol, we consider a static active adversary model. An adversary $\cal A$ can corrupts several participants at the beginning of the protocol and cannot corrupt more participants during the protocol execution. For the corrupted participants, the adversary can see all their received message and directs their actions. Let $\cal C$ denote the participants corrupted by the adversary. (Note that the environment $E$ is not a member of participants and cannot be corrupted.) 

\paragraph{Security analysis} 
We use random variable $\view^{\Pi_\audit}_P({\cal A},pp,\{m_i\}_{i=1}^n,{\cal V})$ for $P\in {\cal P}$ to denote all the received messages of participant $P$ during the execution of the protocol $\Pi_\audit$ with adversary $\cal A$ and the environment setup $\mathsf{Env}(\kappa,k)=(pp,\{m_i\}_{i=1}^n,{\cal V})$. When the context is clear, we use $\view^{\Pi_\audit}_P$ for simplicity. 

First, we show that this protocol leaks no more information than the emission data viewed by the adversary $\cal A$. The adversary can see the emission data for all the corrupted firms. In case the verifier is corrupted, the adversary can also see the emission data of firms in $\cal V$. The theorem~\ref{thm:p1:hiding} proves that the adversary can not learn more information than that. If the country $C$ is corrupted, all the emission data $m_i$ are visible to the adversary and it is unnecessary to discuss the information confidential.

\begin{theorem}\label{thm:p1:hiding}
    There exists a probabilistic polynomial time simulator $\cal S$ such that, if $\cal A$ does not corrupt the country $C$, for any $pp,\{m_i\}_{i=1}^n$ and $\cal V$ setup by the environment $E$,  ${\cal S}\left(pp, m,{\cal V},{\cal M}_F\cup {\cal M}_V\right)$ has the same probability distribution as $\{\view_P({\cal A}, (pp,\{m_i\}_{i=1}^n, {\cal V}))\}_{P\in {\cal C}}$.
    
    Here, ${\cal M}_F$ denote the message $m_i$ for all the corrupted firms $F_i$. ${\cal M}_V$ denotes the message $m_i$ for the picked firms in $\cal V$ if verifier $V$ is corrupted, and equals to $\emptyset$ otherwise.
\end{theorem}
\begin{proof}
    In this proof, we illustrate how a simulator $\cal S$ outputs the view of corrupted participants step by step. We will show that in each step, the simulator's output has the same probability distribution as the received message during the execution of the protocol, conditioned on the output in the previous steps.
    
    Let ${\cal F}_C$ denote the firms corrupted by the adversary, ${\cal F}_V$ denote the firms $\cal V\backslash {\cal F}_C$ in case the verifier is corrupted, and equal to empty set $\emptyset$ otherwise. Let ${\cal F}_H$ denote the firms not in ${\cal F}_C \cup {\cal F}_V$. If ${\cal F}_H$ is not the empty set $\emptyset$, we denote the firm with minimum index by firm $F_m$.
    
    In the step 1, the firm $F_i$ receives messages $m_i$. For each corrupted firm $F_i$ in ${\cal F}_C$, $m_i$ appears in simulator's input and the simulator can simply output it.
    
    In the step 2, all the committed messages $c_i$ are broadcast. For each corrupted firm $F_i$ in ${\cal F}_C$, the simulator outputs $c_i$ by following the adversary's strategy. For each firm $F_i$ in ${\cal F}_V$, the emission data $m_i$ is visible to the simulator. Thus, the simulator samples random $r_i$ from the random value space $\cal R$ and outputs $c_i=\comm_{pp}(m_i,r_i)$. If firm $F_m$ exists, let $m_m=m-\sum_{m_i\in {\cal M}_F\cup {\cal M}_V} m_i$, the simulator samples random $r_m$ and outputs $c_m=\comm_{pp}(m_i,r_i)$. For the other firms $F_i$ in ${\cal F}_H$, the simulator outputs $c_i=\comm_{pp}(0,r_i)$. The unconditional hiding property guarantees that all the simulated committed messages have the same probability distribution as the committed messages during the execution of the protocol. 
    
    In the step 3, the country $C$ examine $c_i=\comm_{pp}(m_i,r_i)$. If the execution of the protocol does not fail at this step, all the examination must pass. Since we do not consider the case that the country is corrupted here, we do not need to discuss the simulator's behaviour.  
    
    In the step 4, the national emission data $m$ and the summation of random value $r$ has been broadcast. Since the examinations at the step 3 have been passed, there must be $\sum_i c_i=\comm_{pp}(m,r)$. The simulator outputs $m$ which appears in the input and $r=\sum_i r_i$ where $r_i$ for each firm $F_i$ are generated in the second step. According to construction of the commitment scheme, given fixed $\sum_i c_i$ and $m$, there exists a unique $r$ satisfying $\sum_i c_i=\comm_{pp}(m,r)$. Thus $r$ has only one possible choice conditioned on $m$ and $\{c_i\}_{i=1}^n$. Since the output of the simulator and the protocol the same probability distribution in the step 2, the $r$ output by the simulator and the protocol must have the same probability distribution. 
    
    In the step 5, the verification set $\cal V$ is broadcast, and the $m_i$ and $r_i$ are forwarded to the verifier. If the verifier is corrupted, the simulator make the verifier receive $m_i$ and $r_i$ for the picked firms in $\cal V$, where $r_i$ is generated in step 2. For the same reason as the step 4, $r_i$ has only one possible choice conditioned on $m_i$ and $c_i$. Thus the $r_i$ outputs by the simulator has the same probability distribution as the $r_i$ in protocol. 
    
    In the step 6 and the step 7, no participant receive messages. So the simulator needs to do nothing. 
    
    Now we have construct a simulator $\cal S$ which makes ${\cal S}\left(pp, m,{\cal V},{\cal M}_F\cup {\cal M}_V\right)$ has the same probability distribution as the participants received messages $\{\view_P\}_{P\in {\cal C}}$ during the execution of the protocol.
\end{proof} 

Second, we show that with a non-negligible probability, the country submits a correct national emission data $m$ or some examinations fail.

\begin{theorem}\label{thm:p1:binding}
    Let $\cal V$ be a random subset of $\{F_i\}_{i=1}^n$ with $k$ elements, 
    $$ \Pr_{\cal V}\left[
    \begin{array}{l}
    m\leftarrow \view^{\Pi_\audit}_{\stat}({\cal A},\stp(1^\kappa),\{m_i\}_{i=1}^n,{\cal V}): \\ 
     m=\bot \;\vee\; m= \sum_{i=1}^m m_i
    \end{array}
    \right]\ge \frac{k}{n}-\mathsf{negl}(\kappa).$$
    
    Here, the random variable $\view^{\Pi_\audit}_{\stat}$ denotes the message $m$ received by the verifier in the step 5 if the execution of protocol successes, and equals to $\bot$ otherwise. 
\end{theorem}
\begin{proof}
    First, we assume the binding property of the commitment scheme is not broken. If $m\neq \bot$, all the examinations must pass. Let $\tilde{m}_i$ denote the self-report emission data submitted from the firm $F_i$ to the country, as long as, there must be $m=\sum_{i=1}^n \tilde{m}_i$. If $\sum_{i=1}^n \tilde{m}_i\neq \sum_{i=1}^n m_i$, there exists as least one firm $F_j$ report the tampered data with $\tilde{m}_j\neq m_j$. If this firm is picked in $\cal V$, the verifier will receive $m_j$ from the environment and the firm $F_j$ can not open the commitment $c_j$ of $\tilde{m}_j$ to another data $m_j$. Thus, the execution will pass only if firm $F_j$ is not included in $\cal V$. Since the set $\cal V$ is revealed after the firm self-reporting data to the country, the firm's action is independent with $\cal V$. So the firm $F_j$ will not be picked in $\cal V$ with probability $\frac{n-k}{n}$.
    
    Since the the binding property of the commitment scheme is broken with probability $\mathsf{negl}(\kappa)$, according to the union bound, we claim 
    $$ \Pr_{\cal V}\left[
    \begin{array}{l}
    m\leftarrow \view^{\Pi_\audit}_{\stat}({\cal A},\stp(1^\kappa),\{m_i\}_{i=1}^n,{\cal V}): \\ 
     m\neq\bot \;\wedge\; m\neq \sum_{i=1}^m m_i
    \end{array}
    \right]\le \frac{n-k}{n}+\mathsf{negl}(\kappa).$$
\end{proof}

\subsection{Random list generation protocol}

The random list generation protocol $\Pi_{\pick}$ consists of an environment $E$ and two participants: the country $C$ and the verifier $V$. Before executing the protocol, the environment $E$ runs the setup algorithm $\stp(1^\kappa)$ for the commitment. The country $C$ and the verifier $V$ has reached agreement for a list of firms $\vec{F}=\{F_i\}_{i=1}^n$ and the number of firms $k$ to be picked.  

\paragraph{Construction}
The execution of the protocol is designed as follows,
\begin{enumerate}
    \item Let $l$ be the length of firm list, the country picks a random integer $m_c$ from $[l]$, encodes it into message space $\cal M$ and compute $c_c=\comm_{pp}(m_c,r_c)$ with random value $r_c$. The verifer computes $c_v$ from $m_v,r_v$ in the same way. 
    \item The country and the verifier send $c_c$ and $c_v$ to each other. 
    \item The country and the verifier send $(m_c,r_c)$ and $(m_v,r_v)$ to each other.
    \item The country examines whether $c_v=\comm_{pp}(m_v,r_v)$. If the examination passes, let $m=m_c+m_v \mbox{ mod } l$. Then it picks the $m$-th firm in the firm list and eliminates it from the list. The verifier does the same thing. 
    \item Repeat the step 1 to the step 4 until $k$ firms are picked. 
\end{enumerate}

At any time the examination fails, the one who provides incorrect data will lose the qualification to participate the protocol. The other one outputs the random list with $k$ element as the output of the protocol. 

\paragraph{Adversary model} In this protocol, we consider a static active adversary model. An adversary $\cal A$ can corrupts one of the country $C$ or the verifier $V$.

\paragraph{Security analysis} 
Let ${\cal V}^{\Pi_\pick}({\cal A}, pp,\vec{F}, k)$ denote the output of protocol $\Pi_\pick$ with the adversary $\cal A$, commitment public parameter $pp$, firm list $\vec{F}$ and the number of picked firms $k$. 

\begin{theorem}
    Let the firm list $\vec{F}$ contain $n$ firms, for any $k$-element set ${\cal V}\subseteq \vec{F}$, it will be 
    $$ \left|\Pr\left[{\cal V}^{\Pi_\pick}({\cal A},\stp(1^\kappa),\vec{F}, k)={\cal V}\right]-\frac{1}{\binom{n}{k}}\right| \le \mathsf{negl}(\kappa).$$
\end{theorem}
\begin{proof}
    First, we assume the binding property of the commitment scheme is not broken. Since the adversary can only corrupt one participant, whenever the adversary makes the corrupted participant send incorrect $m,r$ which can not pass the examination for $c=\comm_{pp}(m,r)$, the honest one must output a truly random subset $\cal V$. 
    
    Now we consider the case that the adversary never make a participant send incorrect $m,r$ in the step 3. Without loss of generality, suppose the adversary corrupts the verifier. At the end of step 2, the verifier has made its decision for $m_v$ but can not see the choice of the country $m_c$. So $m_v$ is independent with country's choice $m_c$. Since $m_c$ is a random integer in $[l]$, $m=m_c+m_v \mbox{ mod } l$ must be random. And thus the eventual firm list must be random. 
    
    With probability $\mathsf{negl}(\kappa)$, the binding property of the commitment scheme will be broken. So the output ${\cal V}^{\Pi_\pick}$ has a negligible distance with a truly random subset.
\end{proof}
